# Supplementary material for: Non-Markovian Stochastic Schr\"odinger Equation: Matrix Product State Approach to the Hierarchy of Pure States
Source: arXiv:2109.06393 source file (2021-12-23)
Supplement: Supplementary file 1 [file HOMPS_SI.pdf]

# Supplementary information: Non-Markovian Stochastic Schrödinger Equation: Matrix Product State Approach to the Hierarchy of Pure States

Xing Gao,[1, a] Jiajun Ren,[2, b] Alexander Eisfeld,[3, c] and Zhigang Shuai[2]

[1] *School of Materials, Sun Yat-sen University, Shenzhen, Guangdong 518107, China*

[2] *MOE Key Laboratory of Organic OptoElectronics and Molecular Engineering, Department of Chemistry, Tsinghua University, Beijing 100084, China*

[3] *Max-Planck-Institut für Physik komplexer Systeme, Nöthnitzer Str. 38, D-01187 Dresden, Germany*

(Dated: 19 November 2021)

## IN THIS SUPPLEMENTAL INFORMATION WE PROVIDE:

**SI. Details on the numerical propagation** 2

**SII. Details about the generation of the stochastic processes** 3

**SIII. Derivation of HOMPS for many coupling operators and multiple bath** 4

**SIV. Details on the molecular aggregate model** 5

A. Additional examples of single trajectories 6

**SV. Alternative way of treating high temperatures** 7

A. Application to the Spin-Boson Model 8

B. Application to the linear chain 9

1. Nearest-neighbor interactions 9

2. Long-range interactions with $V_{jj'} \sim \frac{1}{|j-j'|^3}$ 9

**SVI. Additional convergence tests** 11

A. Spin Boson Model 11

B. Linear chain 11

**References** 12

---

[a] Electronic mail: gxing@mail.sysu.edu.cn

[b] Electronic mail: renjj@mail.tsinghua.edu.cn

[c] Electronic mail: eisfeld@pks.mpg.de

## SI. DETAILS ON THE NUMERICAL PROPAGATION

All calculations were carried out with the open-source package Renormalizer[1] developed by us. We used two propagation algorithms.

(a) An algorithms based on the Runge-Kutta method.

(b) An algorithm based on the time dependent variational principle (TDVP).

For all calculations show in the Letter the Runge kutta based algorithm is used. The results have been validated by the TDVP algorithm.

*a. Runge Kutta:* The MPS/MPO representation of Eq. (9) in the main text is evolved in time according to a global fourth-order Runge-Kutta (RK) algorithm[2] with the noise taken to be constant during a single propagation step. In the process of wavefunction compression, the truncation criteria to retain renormalized states through singular value decomposition is chosen to be $\zeta = 10^{-3}$, *i.e*, only contributions with (normalized) singular value larger than $\zeta$ are taken into account. This implies that the bond dimensions of MPS are adaptively adjusted during the propagation.

*b. TDVP:* We also use the recently developed time dependent variational principle based method with the matrix unfolding and variable mean field (TDVP-MU/VMF) algorithm[2]. In this algorithm, the bond dimension is fixed and the time step size is adaptive choose by Dormand-Prince's 5/4 Runge-Kutta method with a relative tolerance $10^{-3}$ and absolute tolerance $10^{-6}$. The noise is variable in a single time step, different from the above evolution algorithm. It has been found previously that with the same bond dimension $M$, TDVP based evolution algorithm is more accurate than the global RK evolution algorithm.[2] In addition, the algorithm with adaptive time step is more convenient to be used in the unknown systems.

## SII. DETAILS ABOUT THE GENERATION OF THE STOCHASTIC PROCESSES

Stochastic processes that satisfy

$$\begin{aligned} \mathbb{E}[Z_t Z_s] &= 0 \\ \mathbb{E}[Z_t Z_s^*] &= \alpha(t-s) \end{aligned} \tag{S1}$$

with bath correlation function $\alpha(t) = \frac{1}{\pi}\int_0^\infty d\omega J(\omega)\big[\coth(\frac{\beta\omega}{2})\cos\omega t - i\sin\omega t\big]$ are generated in the following form according to Ref. 3,

$$Z(t) = \sum_{j=1}^{N} c_j \Big[\sqrt{\frac{1}{2}\coth\frac{\omega_j\beta}{2} - \frac{1}{2}}e^{i(\omega_j t + 2\pi\phi_{j,1})} + \sqrt{\frac{1}{2}\coth\frac{\omega_j\beta}{2} + \frac{1}{2}}e^{i(-\omega_j t + 2\pi\phi_{j,2})}\Big] \tag{S2}$$

where

$$c_j = \sqrt{\frac{J(\omega_j)\Delta\omega}{\pi}}. \tag{S3}$$

Here, the $\phi_{j,1}$ and $\phi_{j,2}$ are independent random numbers uniformly distributed in $[0,1)$ and $\omega_j = (j - \frac{1}{2})\Delta\omega$. The frequency step $\Delta\omega$ is chosen small enough, and $N$ large enough to ensure that the correlations Eqs. S1 are sufficiently well fulfilled.

## SIII. DERIVATION OF HOMPS FOR MANY COUPLING OPERATORS AND MULTIPLE BATH

In this section we provide the explicit formulas for the case of many coupling operators. As given in Eq. 2 of the main text, the system bath coupling then reads.

$$\hat{H}_{\mathrm{SB}} = \sum_{j=1}^{J} H_{\mathrm{SB},j} = \sum_{j} \hat{L}_j \otimes \sum_{\lambda,j} c_{\lambda,j} \hat{q}_{\lambda,j}. \tag{S4}$$

where each system operator $\hat{L}_j$ couples to its own environment.

$$\hat{H}_{\mathrm{B}} = \sum_{j=1}^{J} \sum_{\lambda} (\frac{\hat{p}_{j\lambda}^2}{2} + \frac{1}{2}\omega_{j\lambda}^2 \hat{q}_{j\lambda}^2) \tag{S5}$$

The linear HOPS equation then becomes

$$\begin{aligned} \partial_t \psi_t^{\mathbf{n}} =& \big[ -i\hat{H}_{\mathrm{S}} + \sum_{j}^{J} \hat{L}_j Z_{t,j}^* - \sum_{j}^{J} \sum_{k=1}^{K} n_{jk} \nu_{jk} \big] \psi_t^{\mathbf{n}} \\ &+ \sum_{j}^{J} \hat{L}_j \sum_{k=1}^{K} \frac{d_{jk}}{\sqrt{|d_{jk}|}} \sqrt{n_{jk}}\, \psi_t^{\mathbf{n}-\mathbf{e}_{jk}} \\ &- \sum_{j}^{J} \hat{L}_j^{\dagger} \sum_{k=1}^{K} \sqrt{|d_{jk}|} \sqrt{n_{jk}+1}\, \psi_t^{\mathbf{n}+\mathbf{e}_{jk}}. \end{aligned} \tag{S6}$$

The corresponding effective Hamiltonian is

$$\begin{aligned} \hat{H}_{\mathrm{eff}} =& \hat{H}_{\mathrm{S}} + i \sum_{j}^{J} \hat{L}_j Z_{t,j}^* - i \sum_{j}^{J} \sum_{k=1}^{K} \nu_{jk} \hat{b}_{jk}^{\dagger} \hat{b}_{jk} \\ &- i \sum_{j}^{J} \sum_{k=1}^{K} [\hat{L}_j^{\dagger} \sqrt{|d_{jk}|} \hat{b}_{jk} - \hat{L}_j \frac{d_{jk}}{\sqrt{|d_{jk}|}} \hat{b}_{jk}^{\dagger}] \end{aligned} \tag{S7}$$

The non-linear equation is obtained making the following replacements:

$$\hat{L}_j^{\dagger} \rightarrow \hat{L}_j^{\dagger} - \langle \hat{L}_j^{\dagger} \rangle_t \tag{S8}$$

$$Z_{t,j}^* \rightarrow Z_{t,j}^* + \int_0^t \mathrm{d}s \alpha_j^*(t-s) \langle \hat{L}_j^{\dagger} \rangle_s \tag{S9}$$

with

$$\langle \hat{L}_j^{\dagger} \rangle_t = \frac{\langle \psi_s^{\mathbf{0}} |\, \hat{L}_j^{\dagger} \,| \psi_s^{\mathbf{0}} \rangle}{\langle \psi_s^{\mathbf{0}} | \psi_s^{\mathbf{0}} \rangle} \ . \tag{S10}$$

## SIV. DETAILS ON THE MOLECULAR AGGREGATE MODEL

In this section we provide in detail the expressions used for the case of molecular aggregates considered in the main text. The connection of this model to molecular aggregates or biological light harvesting systems is discussed e.g., in Refs. 4,5

The system is described by a Hamiltonian

$$\hat{H}_{\mathrm{S}} = \sum_{j=1}^{N} \epsilon_j a_j^\dagger a_j + \sum_{j=1}^{N} \sum_{j' \neq j}^{N} V_{jj'} a_j^\dagger a_{j'} \tag{S11}$$

Each site couples to its own bath, according to Eq. S4 with

$$\hat{L}_j = a_j^\dagger a_j \tag{S12}$$

For nearest neighbor coupling $V_{jj'} \equiv \delta_{j,j'} V$. We also consider long range-interaction with $V_{jj'} \sim \frac{1}{|j-j'|^3}$ which stems from the typical transition dipole-dipole interaction between molecules.

For each environmental mode $(j, k$ and each site $j$ we introduce occupation numbers $s_j$ and $n_{j,k}$. With this we write the MPS representation of state of the HOPS as

$$\begin{aligned} |\Psi\rangle_t &= \sum_{\boldsymbol{s},\mathbf{n}} \psi_t^{\boldsymbol{s},\mathbf{n}} |s_1, n_{11}, \cdots, n_{1K}, \cdots, s_N, n_{N1}, \cdots, n_{NK}\rangle \\ &= \sum_{\boldsymbol{s},\mathbf{n},\mathbf{a}} A^{s_1}_{1,a_{10}} A^{n_{11}}_{a_{10}a_{11}} \cdots A^{n_{NK}}_{a_{NK-1},1} |s_1, n_{11}, \cdots, n_{1K}, s_2, n_{21}, \cdots, s_N, n_{N1}, \cdots, n_{NK}\rangle \,. \end{aligned} \tag{S13}$$

## A. Additional examples of single trajectories

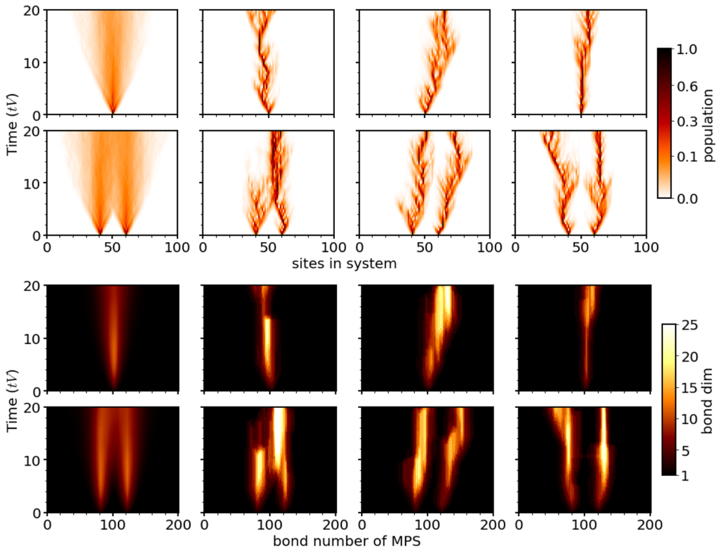


FIG. S1. Populations (*top panel*) and bond dimensions (*bottom panel*) for single trajectories for the parameters of Fig. 3c in the main text. For convenience the first column shows the average over 1000 trajectories.

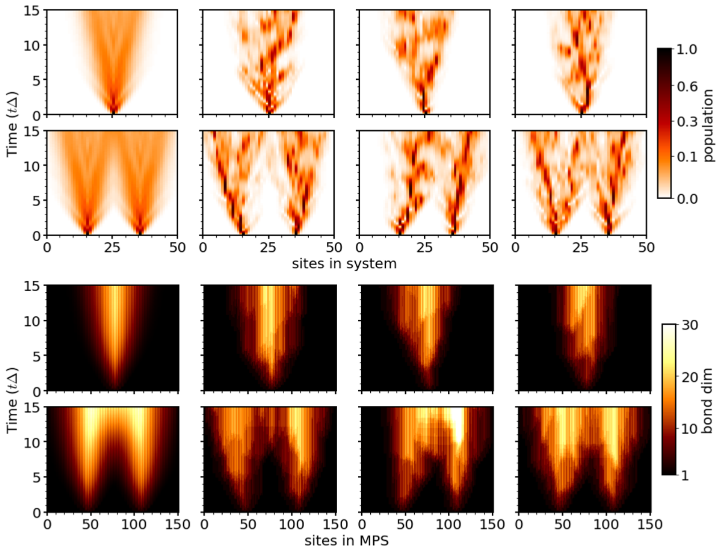


FIG. S2. Same as Fig. S1 but now for the parameters of Fig. 3d of the main text.

## SV. ALTERNATIVE WAY OF TREATING HIGH TEMPERATURES

In general one has some freedom in choosing the exact form of the correlations $\mathbb{E}[Z_t Z_s]$ and $\mathbb{E}[Z_t Z_s^*]$. In the original derivation of NMQSD[6–8], one has $\mathbb{E}[Z_t Z_s] = 0$, $\mathbb{E}[Z_t Z_s^*] = \alpha^*(t-s)$.

Here we want to show that HOMPS also works when using a different form of the correlations, which is in particular suited for high temperature. To this end we consider correlations $\mathbb{E}[Z_t Z_s] = \alpha_1(t-s)$ and $\mathbb{E}[Z_t Z_s^*] = \alpha_2(t-s)$. Of course $\alpha_1(t-s)$ and $\alpha_2(t-s)$ cannot be chosen arbitrarily.

For high temperature, recently the following choice has been advocated [3,9]:

$$\alpha_1(\tau) = \frac{1}{\pi}\int_0^\infty d\omega J(\omega)\ \mathrm{csch}(\frac{\beta\omega}{2})\cos(\omega\tau) \tag{S14}$$

$$\alpha_2(\tau) = \alpha^*(\tau). \tag{S15}$$

The corresponding stochastic processes are generated according to[10]

$$\begin{aligned} Z(t) =& \sum_{j=1}^{N} \sqrt{J(\omega_j)\Delta\omega/\pi} \\ & \times \big[\sqrt{\coth(\frac{\omega_j\beta}{2}) + \mathrm{csch}(\frac{\omega_j\beta}{2})}\cos(\omega_j t + 2\pi\phi_j) \\ & + i\sqrt{\coth(\frac{\omega_j\beta}{2}) - \mathrm{csch}(\frac{\omega_j\beta}{2})}\sin(\omega_j t + 2\pi\phi_j)\big] \end{aligned} \tag{S16}$$

where the $\phi_j$ are independent random numbers uniformly distributed in $[0,1)$.

Starting from the original derivation of NMQSD, we get the following hierarchy of equation,

$$\begin{aligned} \partial_t\psi_t^{\mathbf{n}} =& -\big[i\hat{H}_{\mathrm{S}} + i\sum_j^N \hat{L}_j Z_{t,j} + \sum_j^N\sum_{k=1}^K n_{jk}\nu_{jk}\big]\psi_t^{\mathbf{n}} \\ & -\sum_j^N \hat{L}_j \sum_{k=1}^K \frac{d_{jk}}{\sqrt{|d_{jk}|}}\sqrt{n_{jk}}\,\psi_t^{\mathbf{n}-\mathbf{e}_{jk}} \\ & +\sum_j^N \hat{L}_j^\dagger \sum_{k=1}^K \sqrt{|d_{jk}|}\sqrt{n_{jk}+1}\,\psi_t^{\mathbf{n}+\mathbf{e}_{jk}}. \end{aligned} \tag{S17}$$

which is essentially the same as Eq. S6 but with different definition of noise. The corre-

sponding effective Hamiltonian is,

$$
\begin{aligned}
\hat{H}_{\mathrm{eff}} = \hat{H}_{\mathrm{S}} + \sum_{j}^{N} \hat{L}_j Z_{t,j} - i \sum_{j}^{N} \sum_{k=1}^{K} \nu_{jk} \hat{b}_{jk}^{\dagger} \hat{b}_{jk} \\
+ i \sum_{j}^{N} \sum_{k=1}^{K} [\hat{L}_j^{\dagger} \sqrt{|d_{jk}|} \hat{b}_{jk} - \hat{L}_j \frac{d_{jk}}{\sqrt{|d_{jk}|}} \hat{b}_{jk}^{\dagger}]
\end{aligned} \tag{S18}
$$

## A. Application to the Spin-Boson Model

For proof of principle, we apply the above HOMPS scheme to the SBM, in the the 'high temperature case' of the main text. There we used the non-linear version of HOPS. Here we use the high temperature scheme discussed above, where one can even use the linear version of HOMPS. Using a Matsubara expansion, for the used Debye spectral density one can analytically obtain the exponential decomposition. Inserting the Debye spectral density in the expression of the transformed bath correlation function $\tilde{\alpha}(t) = \frac{1}{\pi} \int_0^{\infty} d\omega J(\omega) \big[ \tanh(\frac{\beta\omega}{4}) \cos\omega t - i \sin\omega t \big]$ and applying the residue theorem, one finds $\nu_1 = \gamma$, $\nu_k = \frac{2\pi}{\beta}(2k-3)$ for $k > 1$, and the corresponding expansion coefficients $d_1 = -\frac{\eta\gamma}{2}\big[\tan(\frac{\beta\gamma}{4}) + i\big]$ and $d_k = -\frac{4\eta\gamma}{\beta}\frac{\nu_k}{\gamma^2 - \nu_k^2}$, $(k > 1)$ . The Markovian terminator can also be calculated analytically $\hat{L}^{\dagger}\hat{L}\Gamma\psi_t^{\mathbf{n}} = \sum_{k=K+1}^{\infty} \frac{d_k}{\nu_k} \hat{L}^{\dagger}\hat{L}\psi_t^{\mathbf{n}} = (\frac{\eta}{2}\tan\frac{\beta\gamma}{4} - \sum_{k=1}^{K}\frac{d_k}{\nu_k})\hat{L}^{\dagger}\hat{L}\psi_t^{\mathbf{n}}$.

In Fig. S3 the population dynamics obtained from HOMPS is shown, where now the linear equation is used. One can see in Fig S3(a), that one has similar good agreement as with the non-linear equation.

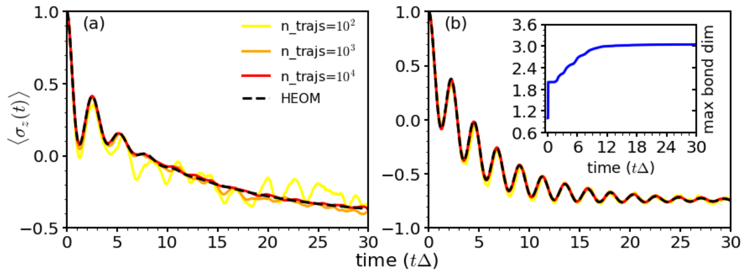


FIG. S3. Population dynamics of spin-boson model with $\epsilon = 1.0$, $\Delta = 1.0$, $\eta = 0.5$ by averaging over $10^2$, $10^3$ and $10^4$ trajectories at (a) high temperature $\beta = 0.5$ and small $\gamma = 0.25$. HOMPS results are obtained using the linear version with $K = 1$ and $n_{\max} = 9$ The reference results are obtained from Ref. 3 where the HEOM method has been used.

### B. Application to the linear chain

#### 1. Nearest-neighbor interactions

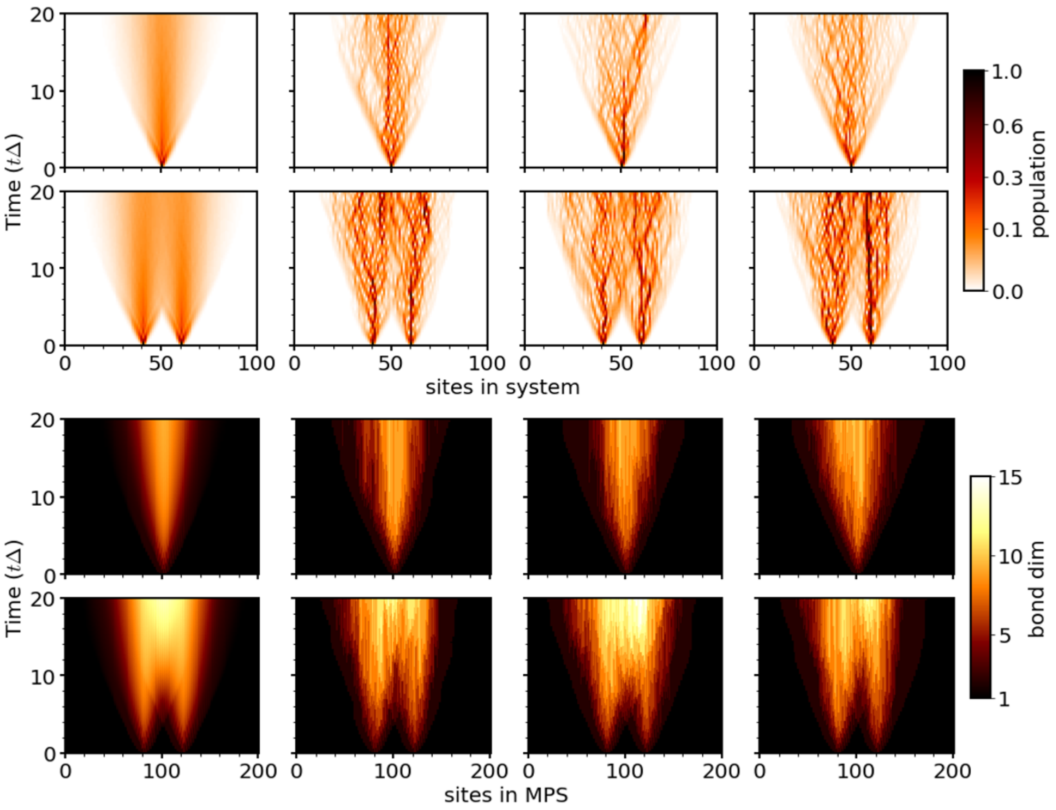


FIG. S4. Evolution of population (*top panel*) and bond dimension (*bottom panel*) for single trajectory using alternative linear HOMPS. The parameters are the same as the high temperature situation in Fig. 3(c) in main text.

#### 2. Long-range interactions with $V_{jj'} \sim \frac{1}{|j-j'|^3}$

Here we show one example of one dimensional chain model including long-range interaction with $V_{jj'} = \frac{1}{|j-j'|^3}$.

To reduce the computational cost, we use (1) alternative linear HOMPS with transformed bath correlaton function for high temperature and (2) evolve the dynamics based on TDVP-MU/VMF propagator with fixed bond dimension $M = 20$. The results are very similar to nearest neighbour case.

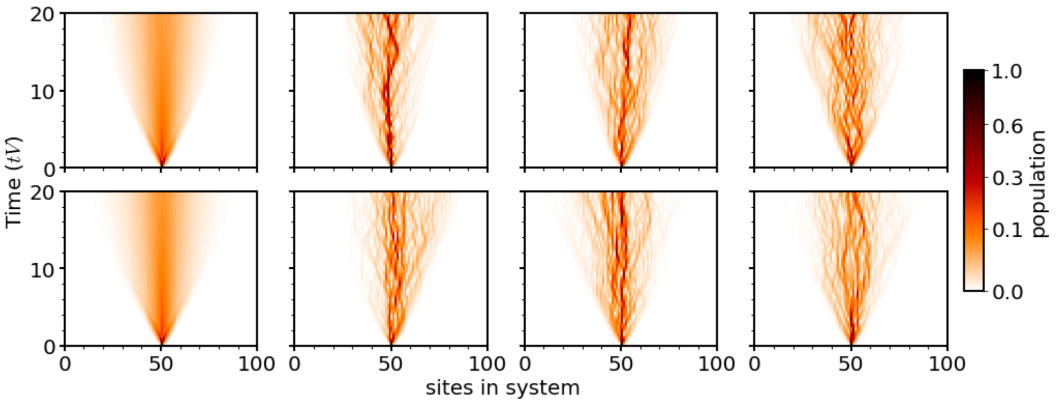


FIG. S5. Evolution of population with nearest-neighbor (*top panel*) and long-range (*bottom panel*) interactions. The first row shows the results averaged over 1000 trajectories. The subsequent panel are examples of single trajectories.

## SVI. ADDITIONAL CONVERGENCE TESTS

### A. Spin Boson Model

Here we check the maximum quantum number needed for each mode in both high and low temperature situation.

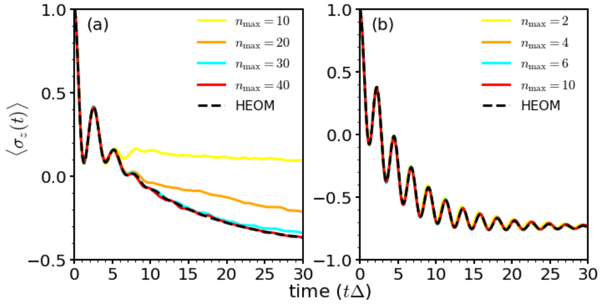


FIG. S6. Evolution of population for (a) high temperature with $n_{\max} = 10,\ 20,\ 30$ and 40, and (b) low temperature, large damping' case, with $n_{\max} = 2,\ 4,\ 6$ and 10. The parameters are the same as Fig. 2 in main text.

### B. Linear chain

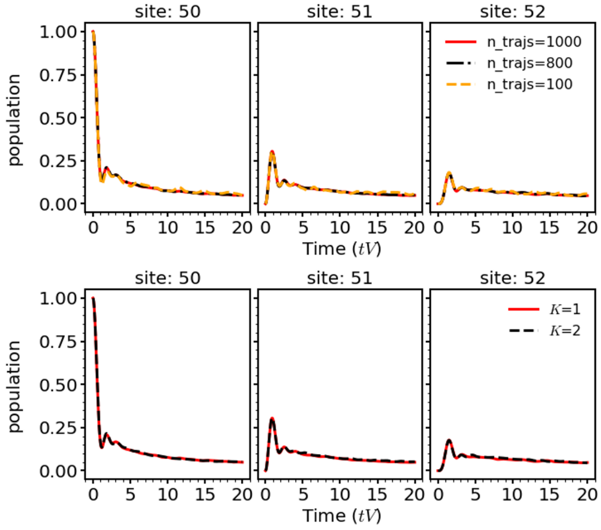


FIG. S7. Top: Evolution of population for different number of trajectories. Bottom: Evolution of population for $K = 1,\ 2$. The parameters are the same as Fig. 3(c) in main text.

## REFERENCES


[1] "Renormalizer," `https://github.com/shuaigroup/Renormalizer`.

[2] W. Li, J. Ren, and Z. Shuai, "Numerical assessment for accuracy and gpu acceleration of td-dmrg time evolution schemes," J. Chem. Phys. **152**, 024127 (2020).

[3] K. Song, L. Song, and Q. Shi, "An alternative realization of the exact non-markovian stochastic schrödinger equation," J. Chem. Phys. **144**, 224105 (2016).

[4] V. May and O. Kühn, *Charge and Energy Transfer Dynamics in Molecular Systems* (John Wiley & Sons, 2008).

[5] H. van Amerongen, L. Valkunas, and R. van Grondelle, *Photosynthetic Excitons* (World Scientific, Singapore, 2000).

[6] L. Diósi and W. T. Strunz, "The non-markovian stochastic schrödinger equation for open systems," Phys. Lett. A **235**, 569–573 (1997).

[7] L. Diósi, N. Gisin, and W. T. Strunz, "Non-markovian quantum state diffusion," Phys. Rev. A **58**, 1699–1712 (1998).

[8] W. T. Strunz, L. Diósi, and N. Gisin, "Open system dynamics with non-markovian quantum trajectories," Phys. Rev. Lett. **82**, 1801 (1999).

[9] Y. Ke and Y. Zhao, "Hierarchy of forward-backward stochastic schrödinger equation," J. Chem. Phys. **145**, 024101 (2016).

[10] X. Zhong and Y. Zhao, "Non-markovian stochastic schrödinger equation at finite temperatures for charge carrier dynamics in organic crystals," J. Chem. Phys. **138**, 014111 (2013).
